# Supplementary material for: Direct and Sparse Deformable Tracking
Source: arXiv:2109.07370 source file (2021-09-15)
Supplement: Supplementary file 1 [file jacobian_equations.tex]

\section{Jacobian derivatives equations}
\label{ap_jacobian}
We develop the equations followed in the implementation of the Jacobians for the optimizations in Eq.~\ref{eq:soft_constrain_error_function}, Eq.~\ref{eq:dt_optimization} and Eq.~\ref{eq:ba_optimization}. To estimate them, we apply the chain rule to each of the residual terms: the photometric error, the deformation energy and the equilibrium point constrain. 

The photometric error was modeled through forward-compositional approach with Eq.~\ref{eq:photometric_error} or as illumination invariant in Eq.~\ref{eq:photometric_error_illu}:
\begin{equation}
    \mathcal{P}^t_i = \sum T(u_p,v_p,k_{\hat{x}},k_{\hat{y}})- I(\pi(\mathbf{T}_{cw} \mathbf{S}^t_i (u_p,v_p)),
    \tag{\ref{eq:photometric_error}}
\end{equation}
and
\begin{equation}
    \mathcal{P}^t_i =  \sum \alpha_i^t T(u_p,v_p) - I(\pi(\mathbf{T}_{cw} \mathbf{S}_i^t(u_p,v_p))- \beta_i^t.
    \tag{\ref{eq:photometric_error_illu}}
\end{equation}

It depends on three groups of parameters: the deformation of the surfel, the camera pose, and the initial parameters. This parameters are optimized depending on the problem.

In the SfT, only the deformation of the surfel is optimized through its translation $\mathbf{t}_i^t$, rotation $\mathbf{R}_i^t$ and the deformation, . The initial parameters of the patch are known and the pose of the camera is fixed $\mathbf{T}_{cw}$.
\begin{equation}
    \mathbf{S}_i^t = (\mathbf{R}_i^t \mathbf{X}_i^0+ \mathbf{t}_i^t) + \mathbf{R}_i^t \mathbf{J}_i^0 \mathbf{F}^t_i \begin{bmatrix}
    \Delta u \\ \Delta v
    \end{bmatrix}
    \tag{\ref{eq:patch3d_movement}}
\end{equation}
The surfel is transformed to the camera reference by:
\begin{equation}
    \mathbf{S}^t_{ic} = \mathbf{T}_{cw}\mathbf{S}^t_i
    \label{eq:rotation}
\end{equation}

{\color{red} no entiendo qué variables incluye $\mathbf{X}$, tampoco entiendo si los incrementos se aplican de forma compositiva}

The derivatives of the photometric error \textit{wrt.} the pose of the camera can be defined through the chain rule:
\begin{equation}
    \frac{\partial \mathcal{P}^t_i}{\partial \mathbf{X}} = -\nabla{I} \frac{\partial \pi}{\partial \mathbf{S}^t_{ic}} \mathbf{R}_{cw} \frac{\partial \mathbf{S}^t_i}{\partial \mathbf{X}} 
    \label{eq:chain_rule_photometric}
\end{equation}
being $\nabla{I}$ the gradient of the image, it is estimated with a central finite differences kernel $\begin{bmatrix}-1 &0& 1 \end{bmatrix}$. $\mathbf{R}_{cw}$ is the rotation of the camera which images the surfel. For the SfT, we assume that the fixed camera is in the origin, so $\mathbf{T}_{cw} = \mathbb{I}_4$.

$\frac{\partial \pi}{\partial \mathbf{S}^t_{ic}}$ is the projection derivative. It is estimated by using the position of the point $\begin{bmatrix}X_c Y_c Z_c\end{bmatrix}^\top$ and the intrinsic calibration of the camera -focal length $f_x, f_y$- in the camera reference as:

\begin{equation}
    \frac{\partial \pi}{\partial {S^t_{ic}}} = \begin{bmatrix} \frac{f_x}{Z_c}& 0 &-\frac{f_x X_c}{Z_c^2}\\
     0 & \frac{f_y}{Z_c} &-\frac{f_y Y_c}{Z_c^2}
    \end{bmatrix}.
\end{equation}

$\frac{\partial \mathbf{S}^t_i}{\partial \mathbf{X}}$ depends on the translation, rotation and deformation of the surfel. The jacobian obtained for this derivative is a $3\times6$ or $3\times9$ matrix.
\begin{equation}
    \frac{\partial \mathbf{S}^t_i}{\partial \mathbf{t_i}} = \mathbb{I}_3.
\end{equation}
\begin{equation}
    \frac{\partial \mathbf{S}^t_i}{\partial \mathbf{R^t_i}} = -[(\mathbf{R}_i^t \mathbf{X}_i^0) + \mathbf{R}_i^t \mathbf{J}_i^0 \mathbf{F}^t_i \begin{bmatrix}
    \Delta u \\ \Delta v
    \end{bmatrix}]_\times
\end{equation}.
\begin{equation}
    \frac{\partial S^t_i}{\partial \mathbf{F^t_i}} = \mathbf{R}^t_i \mathbf{J}_i^0 \begin{bmatrix} \Delta u & 0 & \Delta u \\ 0 & \Delta v & \Delta v \end{bmatrix} .
\end{equation}

For the deformation tracking the camera is not static and its pose is estimated. The derivative of the photometric error \textit{wrt.} the camera motion is:
\begin{equation}
    \frac{\partial \mathcal{P}_i}{\partial T_{cw}} = - \nabla{I} \frac{\partial \pi}{\partial {S^t_i}_c} \begin{bmatrix} \mathbb{I}_3 & -[{S^t_i}_c]_\times
    \end{bmatrix}.
    \label{eq:pose_camera_derivatives}
\end{equation}

Initial parameters are optimized in the bundle adjustment. The texture $T$ is synthesized by projecting the surfel in the reference image with the original position and tangent vectors for each step.
\begin{equation}
    \mathbf{X}_i^0 = \frac{1}{\beta(\hat{x},\hat{y})} \begin{bmatrix} \hat{x}\\\hat{y}\\1
    \end{bmatrix}
    \tag{\ref{eq:position}}
\end{equation}, and
\begin{equation}
    \mathbf{J}_i^0 = \frac{1}{\beta(\hat{x},\hat{y})} \begin{bmatrix} 1 - \hat{x} k_{\hat{x}} & -\hat{x} k_{\hat{y}}\\-\hat{y} k_{\hat{x}} & 1 - \hat{y} k_{\hat{y}}\\-k_{\hat{x}} & -k_{\hat{y}}
    \end{bmatrix}
    \tag{\ref{eq:Jacobian}}
\end{equation},

Each points position are finally estimated as:
\begin{equation}
    \mathbf{S}_i^0 = \mathbf{X}_i^0 + \mathbf{J}_i^0 \begin{bmatrix}
    \Delta u \\ \Delta v
    \end{bmatrix}
    \tag{\ref{eq:patch3d}}
\end{equation},

The position $\mathbf{X}_i^0$ and the jacobian $\mathbf{J}_i^0$ depend linearly on the depth of the surfel $\frac{1}{\beta(\hat{x},\hat{y})}$ . At the same time, the reprojection of the surfel is also proportional to this parameter. That means that the texture of the patch does not depends on the depth, and their derivatives are zero too. In contrast, the texture of the surfel depends on $k_{\hat{x}}$, and $k_{\hat{x}}$. 
\begin{equation}
\begin{split}
    \frac{\partial \mathcal{P}^t_i}{\partial \begin{bmatrix}\beta & k_{\hat{x}}& k_{\hat{y}}\end{bmatrix}} = \nabla{T} \frac{\partial \pi}{\partial {S^0_{ic}}} \frac{\partial S^0_{ic}}{\partial \begin{bmatrix}\beta & k_{\hat{x}}& k_{\hat{y}}\end{bmatrix}}\\
    - \nabla{I} \frac{\partial \pi}{\partial {S^t_{ic}}} R^t_{cw} R^t_{i} R^0_{wc}\frac{\partial S^0_{icr}}{\partial \begin{bmatrix}\beta & k_{\hat{x}}& k_{\hat{y}}\end{bmatrix}}
    \end{split}
    \label{eq:chain_rule_photometric_bk}
\end{equation}
being 
\begin{equation}
\frac{\partial S^0_{icr}}{\partial \begin{bmatrix}\beta & k_{\hat{x}}& k_{\hat{y}}\end{bmatrix}} = \begin{bmatrix}
\frac{\partial S^0_{icr}}{\partial \beta} & \frac{\partial S^0_{icr}}{\partial k_{\hat{x}}} & \frac{\partial S^0_{icr}}{\partial k_{\hat{y}}} 
\end{bmatrix}
\end{equation}.
\begin{equation}
\frac{\partial S^0_{icr}}{\partial \beta} = -\frac{1}{\beta^2} \left(\begin{bmatrix} \hat{x} \\ \hat{y} \\ 1\end{bmatrix} + \begin{bmatrix} 1 - \hat{x} k_{\hat{x}} & -\hat{x} k_{\hat{y}}\\-\hat{y} k_{\hat{x}} & 1 - \hat{y} k_{\hat{y}}\\-k_{\hat{x}} & -k_{\hat{y}}
    \end{bmatrix} \begin{bmatrix} \Delta u\\\Delta v
    \end{bmatrix}\right)
\end{equation},
\begin{equation}
\frac{\partial S^0_{icr}}{\partial k_{\hat{x}}} = -\frac{1}{\beta}\begin{bmatrix}  \hat{x}  & 0\\\hat{y} & 0\\1 & 0
    \end{bmatrix} \begin{bmatrix} \Delta u\\\Delta v
    \end{bmatrix}
\end{equation} and
\begin{equation}
\frac{\partial S^0_{icr}}{\partial k_{\hat{y}}} = -\frac{1}{\beta}\begin{bmatrix}   0 & \hat{x}\\0 & \hat{y}\\0 & 1
    \end{bmatrix} \begin{bmatrix} \Delta u\\\Delta v
    \end{bmatrix}
\end{equation}

$\alpha$ is static and only reestimated at the beginning of the optimization with the initial guess of the coarsest scale. It is enough with multiply $\nabla I$ by the $\alpha$ gain. 

When isometry is soft-constrained, we use a deformation energy to constrain the deformations. Deformation are modeled by the symmetric matrix $\mathbb{F}^t_i$ and the deformation energy is:
\begin{equation}
    \mathcal{I}^t_i = \left\|\mathbf{F}_i^t - \mathbb{I}_2 \right\|_2^2 .
    \tag{\ref{eq:soft_constrain}}
\end{equation}
The derivatives depending to model the deformation energy are:
\begin{equation}
\frac{\partial \mathcal{I}^t_i}{\partial \mathbb{F}} = \mathbb{I}_3
\end{equation}

The equilibrium point has two parametrizations (Eq.~\ref{eq:temporal_consistency} for deformation tracking and Eq.~\ref{eq:equilibrium point_ba} for bundle adjustment). 

For the deformation tracking (Eq.~\ref{eq:temporal_consistency}), the derivatives of the residual are:
\begin{equation}
\frac{\partial \mathcal{E}^t_i}{\partial \mathbf{t}^t_i} = \mathbb{I}_3,
\end{equation}
and to the rotation of the point
\begin{equation}
\frac{\partial \mathcal{E}^t_i}{\partial \mathbf{R}^t_i} = -[{(\mathbf{R}_i^t \mathbf{X}_i^0)}]_\times
\end{equation}

For the bundle adjustment the equations depends on the initial position of the surfels in the first frame and in the rest of frames, following Eq.~\ref{eq:equilibrium point_ba}, 
\begin{equation}
\mathcal{E}^t_i = (\mathbf{X}_i^t - \frac{1}{N_c}\sum_{t} \mathbf{X}_i^t)^\top \sum (\mathbf{X}_i^t - \frac{1}{N_c}\sum_{t} \mathbf{X}_i^t)
    \tag{\ref{eq:equilibrium point_ba}}
\end{equation}.

The derivative of the equilibrium point to the initial position parameters is:
\begin{equation}
\frac{\partial \mathcal{E}^t_i}{\partial \mathbf{t}^t_i} = (1-\frac{1}{N_{c}})\mathbb{I}_3,
\end{equation}
\begin{equation}
\frac{\partial \mathcal{E}^t_i}{\partial \mathbf{t}^t_i} = -(\frac{1}{N_{c}})\mathbb{I}_3,
\end{equation}
\begin{equation}
\frac{\partial \mathcal{E}^t_i}{\partial \mathbf{R}^t_i} = -(1-\frac{1}{N_{c}})[{(\mathbf{R}_i^t \mathbf{X}_i^0)}]_\times
\end{equation}
\begin{equation}
\frac{\partial \mathcal{E}^t_i}{\partial \mathbf{R}^t_i} = (\frac{1}{N_{c}})[{(\mathbf{R}_i^t \mathbf{X}_i^0)}]_\times
\end{equation}
